# Supplementary material for: ACC-ViT : Atrous Convolution's Comeback in Vision Transformers
Source: arXiv:2403.04200 source file (2024-03-07)
Supplement: Supplementary file 1 [file X_suppl.tex]

\clearpage
\setcounter{page}{1}
\maketitlesupplementary

\appendix

\section{Architectural Details}
\begin{strip}
\subsection{Efficient dilated window generation for Atrous Attention using einops}

Our proposed Atrous Attention depends on computing dilated windows efficiently. We have devised a compact einops operation \cite{Rogozhnikov2022Einops:Notation} to partition the images or featuremaps into dilated windows. 

$x-attr1$, $x-attr2$, and $x-attr3$, which are dilated versions of input $x$ with dilation rates of  2, 4, and 8, respectively, can be computed as:

\begin{verbatim}
    x-attr1 = rearrange(x, 'b c (h hs) (w ws) -> (b hs ws) c h w', hs=2, ws=2)
    x-attr2 = rearrange(x, 'b c (h hs) (w ws) -> (b hs ws) c h w', hs=4, ws=4)
    x-attr3 = rearrange(x, 'b c (h hs) (w ws) -> (b hs ws) c h w', hs=8, ws=8)
\end{verbatim}

In our ACC-ViT we consider dilation rates up to 8, therefore it suffices to compute up to $x-attr3$.

This operation effectively extracts $k^2$ dilated windows, partitioned at a dilation rate of $k$. The extracted windows thus can be used for computing windowed attention without any modification to the attention mechanism.

The original image or featuremap can be retrieved from the partitioned windows through a departition operation implemented using the inverse einops operation. 

\begin{verbatim}
    x = rearrange(x-attr1, '(b hs ws) c h w -> b c (h hs) (w ws)', hs=2, ws=2)
    x = rearrange(x-attr2, '(b hs ws) c h w -> b c (h hs) (w ws)', hs=4, ws=4)
    x = rearrange(x-attr3, '(b hs ws) c h w -> b c (h hs) (w ws)', hs=8, ws=8)
\end{verbatim}

\subsection{Overview of the different ACC-ViT layers}

The ACC-ViT layers are based on our proposed Atrous Attention, Atrous Inverted Residual Convolution, and Gating. The convolution operations are identical in all the stages. However. the different stages of ACC-ViT layers use different degrees of Atrous Attention, due to the change in resolution of featuremaps.

\begin{enumerate}[label=(S{{\arabic*}})]
    \item \textbf{Block 1} : Atrous Attention with dilation rates of 2, 4, and 8 are used, along with undilated windowed attention.
    \item \textbf{Block 2} : Atrous Attention with dilation rates of 2, and 4 are used, along with undilated windowed attention.
    \item \textbf{Block 3} : Atrous Attention with a dilation rate of 2 is used, along with undilated windowed attention.
    \item \textbf{Block 4} : Only undilated windowed attention is used.
\end{enumerate}
\end{strip}

\clearpage

\section{Implementation Details}

\begin{strip}

Recent state-of-the-art models make the implementation and trained-weights public. However, the training pipeline script is hardly accessible, which prevents the identical and consistent training of new models. As a result, there have been community efforts to retrain the models using standardized protocols, maintaining reproducibility. TorchVision \cite{TorchVisionmaintainersandcontributors2016TorchVision:Library} and timm \cite{Wightman2019PyTorchModels} are the two most notable open-source projects in this regard.

Our ACC-ViT implementation and ImageNet training pipeline are based on TorchVision v0.15.2 (\url{https://pypi.org/project/torchvision/0.15.2/}). Furthermore, we used the ImageNet-1K trained weights of the baseline models, released by TorchVision. The baseline model weights are summarized in Table \ref{tbl:trchvsn}.

\end{strip}

\begin{table}[]
\centering
\caption{TorchVision weights of baseline models}
\label{tbl:trchvsn}
\begin{tabular}{c|c|c|c|c}
\hline
Model &
  TorchVision weight &
  \begin{tabular}[c]{@{}c@{}}IN-1K Acc\\ (reproduced)\end{tabular} &
  \begin{tabular}[c]{@{}c@{}}IN-1K\\ (published)\end{tabular} &
  Link \\ \hline
Swin &
  Swin\_T\_Weights.IMAGENET1K\_V1 &
  81.474\% &
  81.3\% &
  \begin{tabular}[c]{@{}c@{}}https://download.pytorch.org/models/\\ swin\_t-704ceda3.pth\end{tabular} \\
ConvNeXt &
  ConvNeXt\_Tiny\_Weights.IMAGENET1K\_V1 &
  82.520\% &
  82.1\% &
  \begin{tabular}[c]{@{}c@{}}https://download.pytorch.org/models/\\ convnext\_tiny-983f1562.pth\end{tabular} \\
MaxViT &
  MaxVit\_T\_Weights.IMAGENET1K\_V1 &
  83.7\% &
  83.6\% &
  \begin{tabular}[c]{@{}c@{}}https://download.pytorch.org/models/\\ maxvit\_t-bc5ab103.pth\end{tabular} \\ \hline
\end{tabular}
\end{table}

\clearpage

\section{Experimental Details}

\subsection{ImageNet-1K Training}

\begin{strip}

The ImageNet-1K dataset \cite{Deng2009ImageNet:Database} is a benchmark dataset containing images from 1000 classes. It provides 1.2 million and 50,000 images for training and validation, respectively. We trained the ACC-ViT models mostly based on the TorchVision defaults and the recipe for MaxViT \url{https://github.com/pytorch/vision/tree/main/references/classification#maxvit} and trained the models for 400 epochs with cosine annealing learning rate scheduler and exponential moving average (EMA). The batch size and learning rate were adjusted based on the computational limitations set by GPU memory. Taking inspiration from FocalNet \cite{Yang2022FocalNetworks} we considered both cutmix \cite{Yun2019CutMix:Features} and mixup \cite{Zhang2017Mixup:Minimization} augmentations.

The training hyperparameters are summarized in table \ref{tbl:hypimg}.
\end{strip}

\begin{table}[h]
\centering
\caption{Hyperparameters for ImageNet training}
\label{tbl:hypimg}
\begin{tabular}{c|ccccc}
\hline
Hyperparameter        & femto    & pico    & nano    & tiny    & small    \\ \hline
image resolution      & \multicolumn{5}{c}{$224 \times 224$} \\
batch size            & 3072     & 2560    & 2048    & 1024    & 768      \\
stochastic depth      & 0.0      & 0.0     & 0.1     & 0.2     & 0.3      \\
learning rate         & 1e-3     & 1e-3    & 1e-3    & 1e-3    & 5e-4     \\
min learning rate     & 1e-5     & 1e-5    & 1e-5    & 1e-5    & 5e-6     \\
training epochs       & \multicolumn{5}{c}{400}                           \\
warm-up epochs       & \multicolumn{5}{c}{32}                           \\
Optimizer             & \multicolumn{5}{c}{adamw}                         \\
schedular             & \multicolumn{5}{c}{cosine annealing}              \\
loss function         & \multicolumn{5}{c}{softmax}                       \\
randaugment policy    & \multicolumn{5}{c}{ta-wide}                       \\
randaugment magnitude & \multicolumn{5}{c}{15}                            \\
randaugment sampler   & \multicolumn{5}{c}{3}                             \\
cutmix-alpha          & \multicolumn{5}{c}{0.8}                           \\
mixup-alpha           & \multicolumn{5}{c}{0.8}                           \\
label-smoothing       & \multicolumn{5}{c}{0.1}                           \\
gradient clip         & \multicolumn{5}{c}{1.0}                           \\
ema steps             & \multicolumn{5}{c}{32}                          \\ \hline 
\end{tabular}
\end{table}

\clearpage

\begin{strip}

The detailed training commands of the ACC-ViT models, based on TorchVision are as follows:

\begin{itemize}

\item ACC-ViT femto

\begin{verbatim}
CUBLAS_WORKSPACE_CONFIG=:16:8 torchrun --nproc-per-node=16 --nnodes=1 train.py 
--model accvit_f --epochs 400 --batch-size 192 --opt adamw --lr 1e-3 
--weight-decay 0.05 --lr-scheduler cosineannealinglr --lr-min 1e-5 
--lr-warmup-method linear --lr-warmup-epochs 32 --label-smoothing 0.1 
--mixup-alpha 0.8 --cutmix-alpha 0.8 --clip-grad-norm 1.0 --interpolation bicubic 
--auto-augment ta_wide --ra-magnitude 15 --ra-sampler --model-ema 
--val-resize-size 224 --val-crop-size 224 --train-crop-size 224 
--model-ema-steps 32 --transformer-embedding-decay 0 --amp 
--use-deterministic-algorithms --sync-bn 
--data-path ../../../imagenet_full/ILSVRC/Data/CLS-LOC/ 
--output-dir accvit_femto_imgnet_1k
\end{verbatim}

    \item ACC-ViT pico
\begin{verbatim}
CUBLAS_WORKSPACE_CONFIG=:16:8 torchrun --nproc-per-node=16 --nnodes=1 train.py 
--model accvit_p --epochs 400 --batch-size 160 --opt adamw --lr 1e-3 
--weight-decay 0.05 --lr-scheduler cosineannealinglr --lr-min 1e-5 
--lr-warmup-method linear --lr-warmup-epochs 32 --label-smoothing 0.1
--mixup-alpha 0.8 --cutmix-alpha 0.8 --clip-grad-norm 1.0 --interpolation bicubic
--auto-augment ta_wide --ra-magnitude 15 --ra-sampler --model-ema
--val-resize-size 224 --val-crop-size 224 --train-crop-size 224 
--model-ema-steps 32 --transformer-embedding-decay 0 --amp 
--use-deterministic-algorithms --sync-bn 
--data-path ../../../imagenet_full/ILSVRC/Data/CLS-LOC/ 
--output-dir accvit_pico_imgnet_1k
\end{verbatim}

\item ACC-ViT nano
\begin{verbatim}
CUBLAS_WORKSPACE_CONFIG=:16:8 torchrun --nproc-per-node=16 --nnodes=1 train.py 
--model accvit_n --epochs 400 --batch-size 128 --opt adamw --lr 1e-3 
--weight-decay 0.05 --lr-scheduler cosineannealinglr --lr-min 1e-5
--lr-warmup-method linear --lr-warmup-epochs 32 --label-smoothing 0.1
--mixup-alpha 0.8 --cutmix-alpha 0.8 --clip-grad-norm 1.0 --interpolation bicubic
--auto-augment ta_wide --ra-magnitude 15 --ra-sampler --model-ema
--val-resize-size 224 --val-crop-size 224 --train-crop-size 224 
--model-ema-steps 32 --transformer-embedding-decay 0 --amp 
--use-deterministic-algorithms --sync-bn
--data-path ../../../imagenet_full/ILSVRC/Data/CLS-LOC/ 
--output-dir accvit_nano_imgnet_1k
\end{verbatim}

\item ACC-ViT tiny
\begin{verbatim}
CUBLAS_WORKSPACE_CONFIG=:16:8 torchrun --nproc-per-node=16 --nnodes=1 train.py
--model accvit_t --epochs 400 --batch-size 64 --opt adamw --lr 1e-3
--weight-decay 0.05 --lr-scheduler cosineannealinglr --lr-min 1e-5
--lr-warmup-method linear --lr-warmup-epochs 32 --label-smoothing 0.1
--mixup-alpha 0.8 --cutmix-alpha 0.8 --clip-grad-norm 1.0 --interpolation bicubic
--auto-augment ta_wide --ra-magnitude 15 --ra-sampler --model-ema
--val-resize-size 224 --val-crop-size 224 --train-crop-size 224 
--model-ema-steps 32 --transformer-embedding-decay 0 --amp
--use-deterministic-algorithms --sync-bn
--data-path ../../../imagenet_full/ILSVRC/Data/CLS-LOC/
--output-dir accvit_tiny_imgnet_1k
\end{verbatim}

\item ACC-ViT small

\begin{verbatim}
CUBLAS_WORKSPACE_CONFIG=:16:8 torchrun --nproc-per-node=16 --nnodes=1  train.py
--model accvit_s --epochs 400 --batch-size 48 --opt adamw --lr 5e-4
--weight-decay 0.05 --lr-scheduler cosineannealinglr --lr-min 5e-6
--lr-warmup-method linear --lr-warmup-epochs 32 --label-smoothing 0.1 
--mixup-alpha 0.8 --cutmix-alpha 0.8 --clip-grad-norm 1.0 --interpolation bicubic 
--auto-augment ta_wide --ra-magnitude 15 --ra-sampler --model-ema 
--val-resize-size 224 --val-crop-size 224 --train-crop-size 224 
--model-ema-steps 32 --transformer-embedding-decay 0 --amp 
--use-deterministic-algorithms --sync-bn 
--data-path ../../../imagenet_full/ILSVRC/Data/CLS-LOC/ 
--output-dir accvit_small_imgnet_1k
\end{verbatim}

\end{itemize}

\subsection{Finetuning on Medical Image Datasets}

In order to assess the transferability of the learned visual representations, we experimented on 3 medical image datasets of different modalities and sizes.

\begin{enumerate}
    \item \textbf{HAM10000} : The HAM10000 \cite{Tschandl2018TheLesions} dataset contains 10,015 dermatoscopic images from 7 different classes of pigmented skin lesions. The 7 classes are akiec (actinic keratoses and intraepithelial carcinomae), bcc (basal cell carcinoma), bkl (benign keratosis-like lesions), df (dermatofibroma), nv (melanocytic nevi), vasc (pyogenic granulomas and hemorrhage) and mel (melanoma). This dataset is quite imbalanced, nearly $2/3^{rd}$ of the images belong to the nv class, whereas akiec, df and vasc comprises $3.25\%$, $1.15\%$, and $1.4\%$, of the dataset respectively.

    \item \textbf{EyePACS} : The EyePACS dataset \cite{Cuadros2009EyePACS:Screening} is a source of high-resolution retina images taken under a variety of imaging conditions. In our experiments, we considered the 5,000 images of this dataset used for training in the Diabetic Retinopathy Detection competition, held at Kaggle (\url{https://www.kaggle.com/competitions/diabetic-retinopathy-detection/data}). The retinal images in this dataset are annotated into 5 grades of diabetic retinopathy, starting from none, spread to mild, moderate, severe, and up to proliferative level of diabetic retinopathy. This dataset is quite imbalanced as well, as almost $3/4^{th}$ of the retinal images have no diabetic retinopathy.

    \item \textbf{BUSI} : The BUSI dataset \cite{Al-Dhabyani2020DatasetImages} is a dataset of 780 breast ultrasound images from 600 patients. The images are categorized into 3 classes, namely, normal, benign, and malignant.
\end{enumerate}

We randomly partitioned the datasets into 60-20-20 train-validation-test splits. The models were fine-tuned using the training split and based on the validation loss the best checkpoints were obtained. Finally, the performance on the test split was assessed.

We adopted the finetuning strategy of MaxViT \cite{Tu2022MaxViT:Transformer} to finetune ACC-ViT and the baseline models on the medical image datasets. The learning rate was set to $5e^{-5}$ without any scheduler or warm-up. Other than RandAugment no other augmentation strategy, i.e., cutmix or mixup, was used. The values of label smoothing and gradient were set to 0.1 and 1.0, respectively. We finetuned the models for 100 epochs, longer than the usual 30 epochs. ACC-ViT managed to finetune rather quickly whereas MaxViT took longer on the medical images.

\subsection{Frozen Backbone Assessment on Object Detection }
The MS-COCO dataset contains 118k training and 5k validation images. Our experiments on this dataset is based on the default config of mmdetection \cite{Chen2019MMDetection:Benchmark}. We used the base configs of mask-rcnn\_r50\_fpn model and coco\_instance dataset. The models were trained using the base config of schedule\_1x and the default\_runtime was followed.

The config followed by ACC-ViT and the baseline models is as follows:

\begin{verbatim}
    

_base_ = [
    '../_base_/models/mask-rcnn_r50_fpn.py',
    '../_base_/datasets/coco_instance.py',
    '../_base_/schedules/schedule_1x.py', '../_base_/default_runtime.py'
]

model = dict(
    type='MaskRCNN',
    backbone=dict(
        type='AccVit'
        ),
    neck=dict(in_channels=[64, 128, 256, 512]))

max_epochs = 12
train_cfg = dict(max_epochs=max_epochs)

train_pipeline = [
    dict(type='LoadImageFromFile'),
    dict(type='LoadAnnotations', with_bbox=True, with_mask=True),
    dict(type='RandomFlip', prob=0.5),
    dict(type='Resize', scale=(224, 224), keep_ratio=True),
    dict(type='Pad', pad_to_square=True),
    dict(type='PackDetInputs')
]
test_pipeline = [
    dict(type='LoadImageFromFile'),    
    dict(type='LoadAnnotations', with_bbox=True, with_mask=True),
    dict(type='Resize', scale=(224, 224), keep_ratio=True),
    dict(type='Pad', pad_to_square=True),
    dict(
        type='PackDetInputs',
        meta_keys=('img_id', 'img_path', 'ori_shape', 'img_shape',
                   'scale_factor'))
]
train_dataloader = dict(
    batch_size=12,
    num_workers=6,
    persistent_workers=True,
    sampler=dict(type='DefaultSampler', shuffle=True),
    batch_sampler=dict(type='AspectRatioBatchSampler'),
    dataset=dict(
        pipeline=train_pipeline))
val_dataloader = dict(
    batch_size=12,
    num_workers=6,
    persistent_workers=True,
    drop_last=False,
    sampler=dict(type='DefaultSampler', shuffle=False),
    dataset=dict(
        pipeline=test_pipeline))
test_dataloader = val_dataloader

param_scheduler = [
    dict(
        type='LinearLR', start_factor=0.001, by_epoch=False, begin=0,
        end=1000),
    dict(
        type='MultiStepLR',
        begin=0,
        end=max_epochs,
        by_epoch=True,
        milestones=[8, 11],
        gamma=0.1)
]

optim_wrapper = dict(
    type='OptimWrapper',
    paramwise_cfg=dict(
        custom_keys={
            'absolute_pos_embed': dict(decay_mult=0.),
            'relative_position_bias_table': dict(decay_mult=0.),
            'norm': dict(decay_mult=0.)
        }),
    optimizer=dict(
        _delete_=True,
        type='AdamW',
        lr=0.0001,
        betas=(0.9, 0.999),
        weight_decay=0.05))

\end{verbatim}

\subsection{Zero-shot Assessment on ELEVATER benchmark}

We used the official GitHub release (\url{https://github.com/Computer-Vision-in-the-Wild/Elevater_Toolkit_IC)} of the ELEVATER benchmark \cite{Li2022ELEVATER:Models}. More specifically, our experiments were conducted on the commit \url{00d0af78559d5f3d800ae4668210e6bd1f2f84b9}. Following the default specification, we used the CLIP ViT/B-32 checkpoint. We developed the visual feature extractor based on the example of swin transformer available at \url{https://github.com/Computer-Vision-in-the-Wild/Elevater_Toolkit_IC/blob/main/vision_benchmark/models/clip_swin.py}.

Due to the stochastic nature of the uninitialized and untrained zero-shot experiments of this benchmark, we ran 3 random experiments for each of the models and considered the mean performance.

\section{Detailed Results}

\subsection{Finetuning on Medical Images}

Here, we present the detailed class-wise metrics and confusion matrices of the different models on the three different datasets.

From the overall results, a few points can be observed. 

\begin{enumerate}
    \item Across all the datasets, ACC-ViT predictions were consistently precise, which is evident from the highest precision scores.
    \item ACC-ViT has demonstrated a poor recall on the \textit{normal} class of the BUSI dataset, which has affected the overall score on that dataset. However, for the most important class of that dataset, i.e., \textit{malignent}, ACC-ViT actually managed to score the highest recall, $4.76\%$ higher than the best-performing ConvNeXt model.
    \item Notably, for the difficult \textit{mild} class of the EyePACS dataset ACC-ViT resulted in the highest recall, which is twice the second best method.
    \item MaxViT struggled quite a bit in predicting the rare classes. For example, it failed to classify any images of the df class from the HAM10000 dataset correctly.
\end{enumerate}

\subsection{Zero-shot Performance on ELEVATER Benchmark}

The individual scores of each of the 3 random trials on the ELEVATER benchmark are presented in Table \ref{tbl:szero}. It can be observed that ACC-ViT outperformed the baseline models in the majority of the experiments.

\end{strip}
