# Supplementary material for: ACC-ViT : Atrous Convolution's Comeback in Vision Transformers
Source: arXiv:2403.04200 source file (2024-03-07)
Supplement: Supplementary file 2 [file X_suppl2.tex]

\begin{table*}[h]
\caption{Detailed results on the HAM10000 dataset}
\label{tbl:sham}
\footnotesize
\begin{tabular}{c|ccc|ccc|ccc|ccc|c}
\hline
               & \multicolumn{3}{c|}{ACC-ViT} & \multicolumn{3}{c|}{ConvNeXt} & \multicolumn{3}{c|}{Swin}   & \multicolumn{3}{c|}{MaxViT} &      \\
 &
  precision &
  recall &
  f1-score &
  precision &
  recall &
  f1-score &
  precision &
  recall &
  f1-score &
  precision &
  recall &
  f1-score &
  count \\ \hline
\textbf{akiec} & 0.8235  & 0.6462  & 0.7241  & 0.7069   & 0.6308  & 0.6667  & 0.7358  & 0.6000  & 0.6610 & 0.6857  & 0.3692  & 0.4800 & 65   \\
\textbf{bcc}   & 0.8785  & 0.9126  & 0.8952  & 0.8034   & 0.9126  & 0.8545  & 0.7851  & 0.9223  & 0.8482 & 0.6791  & 0.8835  & 0.7679 & 103  \\
\textbf{bkl}   & 0.8545  & 0.8545  & 0.8545  & 0.8586   & 0.7455  & 0.7981  & 0.8503  & 0.7227  & 0.7813 & 0.7026  & 0.7409  & 0.7212 & 220  \\
\textbf{df}    & 1.0000  & 0.7826  & 0.8780  & 0.8571   & 0.5217  & 0.6486  & 0.8667  & 0.5652  & 0.6842 & 0.0000  & 0.0000  & 0.0000 & 23   \\
\textbf{mel}   & 0.7860  & 0.8072  & 0.7965  & 0.7708   & 0.6637  & 0.7133  & 0.7031  & 0.6054  & 0.6506 & 0.6378  & 0.5291  & 0.5784 & 223  \\
\textbf{nv}    & 0.9586  & 0.9664  & 0.9625  & 0.9330   & 0.9761  & 0.9541  & 0.9260  & 0.9709  & 0.9479 & 0.9171  & 0.9567  & 0.9365 & 1341 \\
\textbf{vasc}  & 1.0000  & 0.9286  & 0.9630  & 0.9286   & 0.9286  & 0.9286  & 0.8966  & 0.9286  & 0.9123 & 0.8889  & 0.5714  & 0.6957 & 28   \\\hline
\begin{tabular}[c]{@{}c@{}}macro\\ avg\end{tabular} &
  0.9002 &
  0.8426 &
  0.8677 &
  0.8369 &
  0.7684 &
  0.7948 &
  0.8234 &
  0.7593 &
  0.7837 &
  0.6445 &
  0.5787 &
  0.5971 &
   \\
\begin{tabular}[c]{@{}c@{}}weighted\\ avg\end{tabular} &
  0.9205 &
  0.9206 &
  0.9200 &
  0.8918 &
  0.8957 &
  0.8918 &
  0.8784 &
  0.8832 &
  0.8786 &
  0.8318 &
  0.8462 &
  0.8354 &
   \\\hline
accuracy       & \multicolumn{3}{c|}{0.9206}  & \multicolumn{3}{c|}{0.8957}   & \multicolumn{3}{c|}{0.8832} & \multicolumn{3}{c|}{0.8462} &  \\ \hline   
\end{tabular}
\end{table*}

\begin{table*}[h]
\caption{Detailed results on the EyePACS dataset}
\label{tbl:sye}
\footnotesize
\begin{tabular}{c|ccc|ccc|ccc|ccc|c}
\hline
                       & \multicolumn{3}{c|}{ACC-ViT}   & \multicolumn{3}{c|}{ConvNeXt}  & \multicolumn{3}{c|}{Swin}      & \multicolumn{3}{c|}{MaxViT}    &       \\ \hline
                       & precision & recall & f1-score & precision & recall & f1-score & precision & recall & f1-score & precision & recall & f1-score & count \\ \hline
\textbf{none}         & 0.8970    & 0.9698 & 0.9320   & 0.8753    & 0.9766 & 0.9232   & 0.8626    & 0.9781 & 0.9167   & 0.8733    & 0.9804 & 0.9238   & 5162  \\
\textbf{mild}          & 0.4577    & 0.1881 & 0.2667   & 0.4839    & 0.0920 & 0.1546   & 0.5000    & 0.0348 & 0.0650   & 0.4894    & 0.0470 & 0.0858   & 489   \\
\textbf{moderate}      & 0.7269    & 0.6843 & 0.7050   & 0.7048    & 0.6295 & 0.6650   & 0.6812    & 0.6059 & 0.6413   & 0.6974    & 0.6144 & 0.6533   & 1058  \\
\textbf{severe}        & 0.5526    & 0.3600 & 0.4360   & 0.5271    & 0.3886 & 0.4474   & 0.5046    & 0.3143 & 0.3873   & 0.4929    & 0.3943 & 0.4381   & 175   \\
\textbf{proliferative} & 0.6866    & 0.6479 & 0.6667   & 0.7500    & 0.5282 & 0.6198   & 0.8202    & 0.5141 & 0.6320   & 0.6786    & 0.5352 & 0.5984   & 142   \\ \hline
\begin{tabular}[c]{@{}c@{}}macro\\ avg\end{tabular}    & 0.6642 & 0.5700 & 0.6012 & 0.6682 & 0.5230 & 0.5620 & 0.6737 & 0.4894 & 0.5285 & 0.6463 & 0.5143 & 0.5399 &  \\
\begin{tabular}[c]{@{}c@{}}weighted\\ avg\end{tabular} & 0.8280 & 0.8507 & 0.8338 & 0.8112 & 0.8390 & 0.8128 & 0.8003 & 0.8305 & 0.7971 & 0.8067 & 0.8367 & 0.8061 &  \\ \hline
accuracy               & \multicolumn{3}{c|}{0.8507}    & \multicolumn{3}{c|}{0.8390}    & \multicolumn{3}{c|}{0.8305}    & \multicolumn{3}{c|}{0.8367}    &   \\ \hline   
\end{tabular}
\end{table*}

\begin{table*}[h]
\caption{Detailed results on the BUSI dataset}
\label{tbl:sbusi}
\footnotesize
\begin{tabular}{c|ccc|ccc|ccc|ccc|c}
\hline
                   & \multicolumn{3}{c|}{ACC-ViT}   & \multicolumn{3}{c|}{ConvNeXt}  & \multicolumn{3}{c|}{Swin}      & \multicolumn{3}{c|}{MaxViT}    &       \\ \hline
                   & precision & recall & f1-score & precision & recall & f1-score & precision & recall & f1-score & precision & recall & f1-score & count \\\hline
\textbf{benign}    & 0.8261    & 0.8736 & 0.8492   & 0.8539    & 0.8736 & 0.8636   & 0.8161    & 0.8161 & 0.8161   & 0.7358    & 0.8966 & 0.8083   & 87    \\
\textbf{malignent} & 0.7674    & 0.7857 & 0.7765   & 0.8611    & 0.7381 & 0.7949   & 0.8333    & 0.7143 & 0.7692   & 0.7273    & 0.5714 & 0.6400   & 42    \\
\textbf{normal}    & 0.8095    & 0.6296 & 0.7083   & 0.6774    & 0.7778 & 0.7241   & 0.6061    & 0.7407 & 0.6667   & 0.7059    & 0.4444 & 0.5455   & 27    \\\hline
\begin{tabular}[c]{@{}c@{}}macro\\ avg\end{tabular}    & 0.8010 & 0.7630 & 0.7780 & 0.7975 & 0.7965 & 0.7942 & 0.7518 & 0.7570 & 0.7507 & 0.7230 & 0.6375 & 0.6646 &  \\
\begin{tabular}[c]{@{}c@{}}weighted\\ avg\end{tabular} & 0.8074 & 0.8077 & 0.8052 & 0.8253 & 0.8205 & 0.8210 & 0.7844 & 0.7756 & 0.7776 & 0.7284 & 0.7308 & 0.7175 &  \\\hline
accuracy           & \multicolumn{3}{c|}{0.8077}    & \multicolumn{3}{c|}{0.8205}    & \multicolumn{3}{c|}{0.7756}    & \multicolumn{3}{c|}{0.7308}    &  \\ \hline    
\end{tabular}
\end{table*}

\begin{figure*}[h]
     \centering
     \begin{subfigure}[b]{0.99\textwidth}
         \centering
         \includegraphics[width=\textwidth]{author-kit-CVPR2024-v2/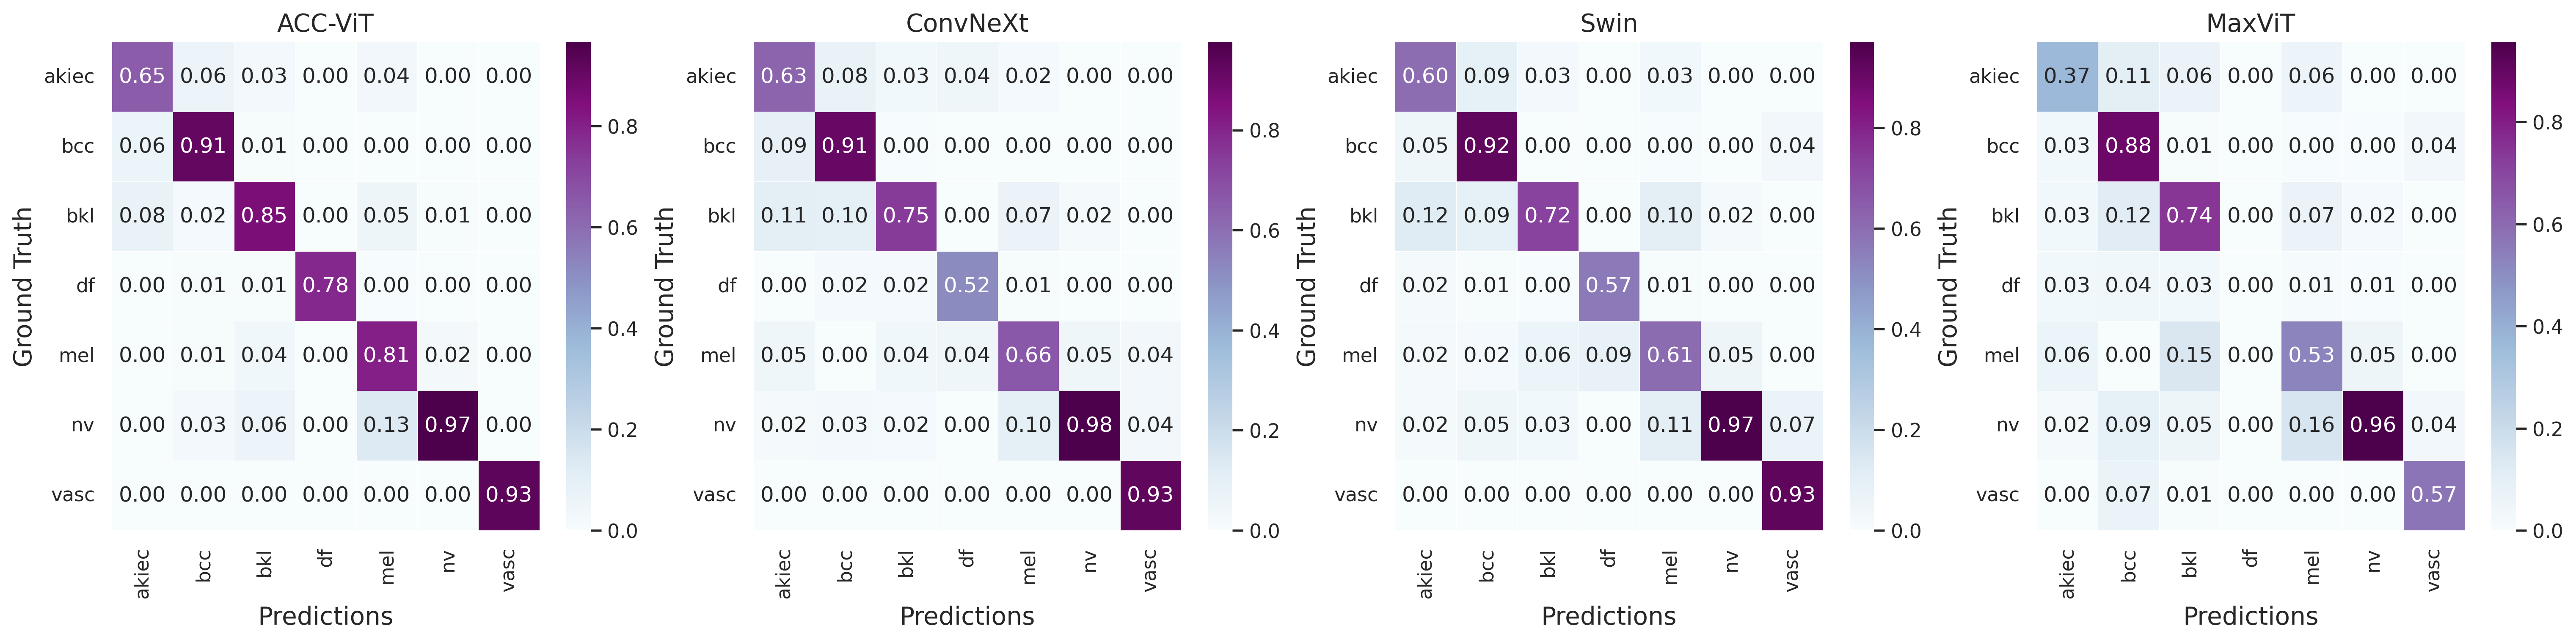}
         \caption{HAM10000 dataset}
     \end{subfigure}
     \hfill
     \begin{subfigure}[b]{0.99\textwidth}
         \centering
         \includegraphics[width=\textwidth]{author-kit-CVPR2024-v2/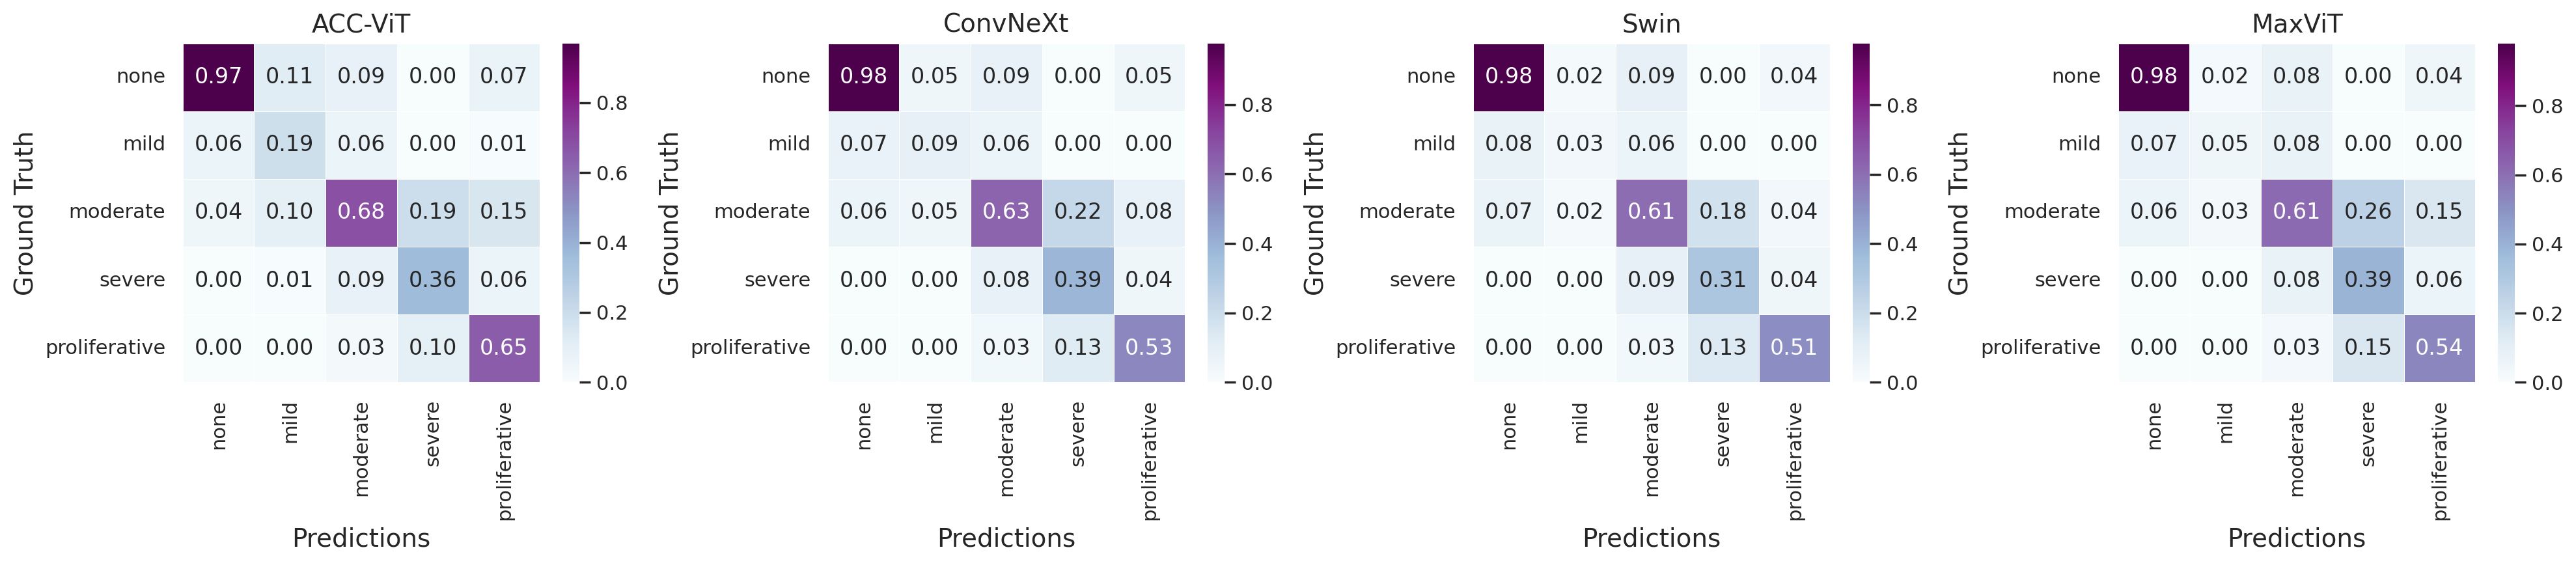}
         \caption{EyePACS dataset}
     \end{subfigure}
     \hfill
     \begin{subfigure}[b]{0.7\textwidth}
         \centering
         \includegraphics[width=\textwidth]{author-kit-CVPR2024-v2/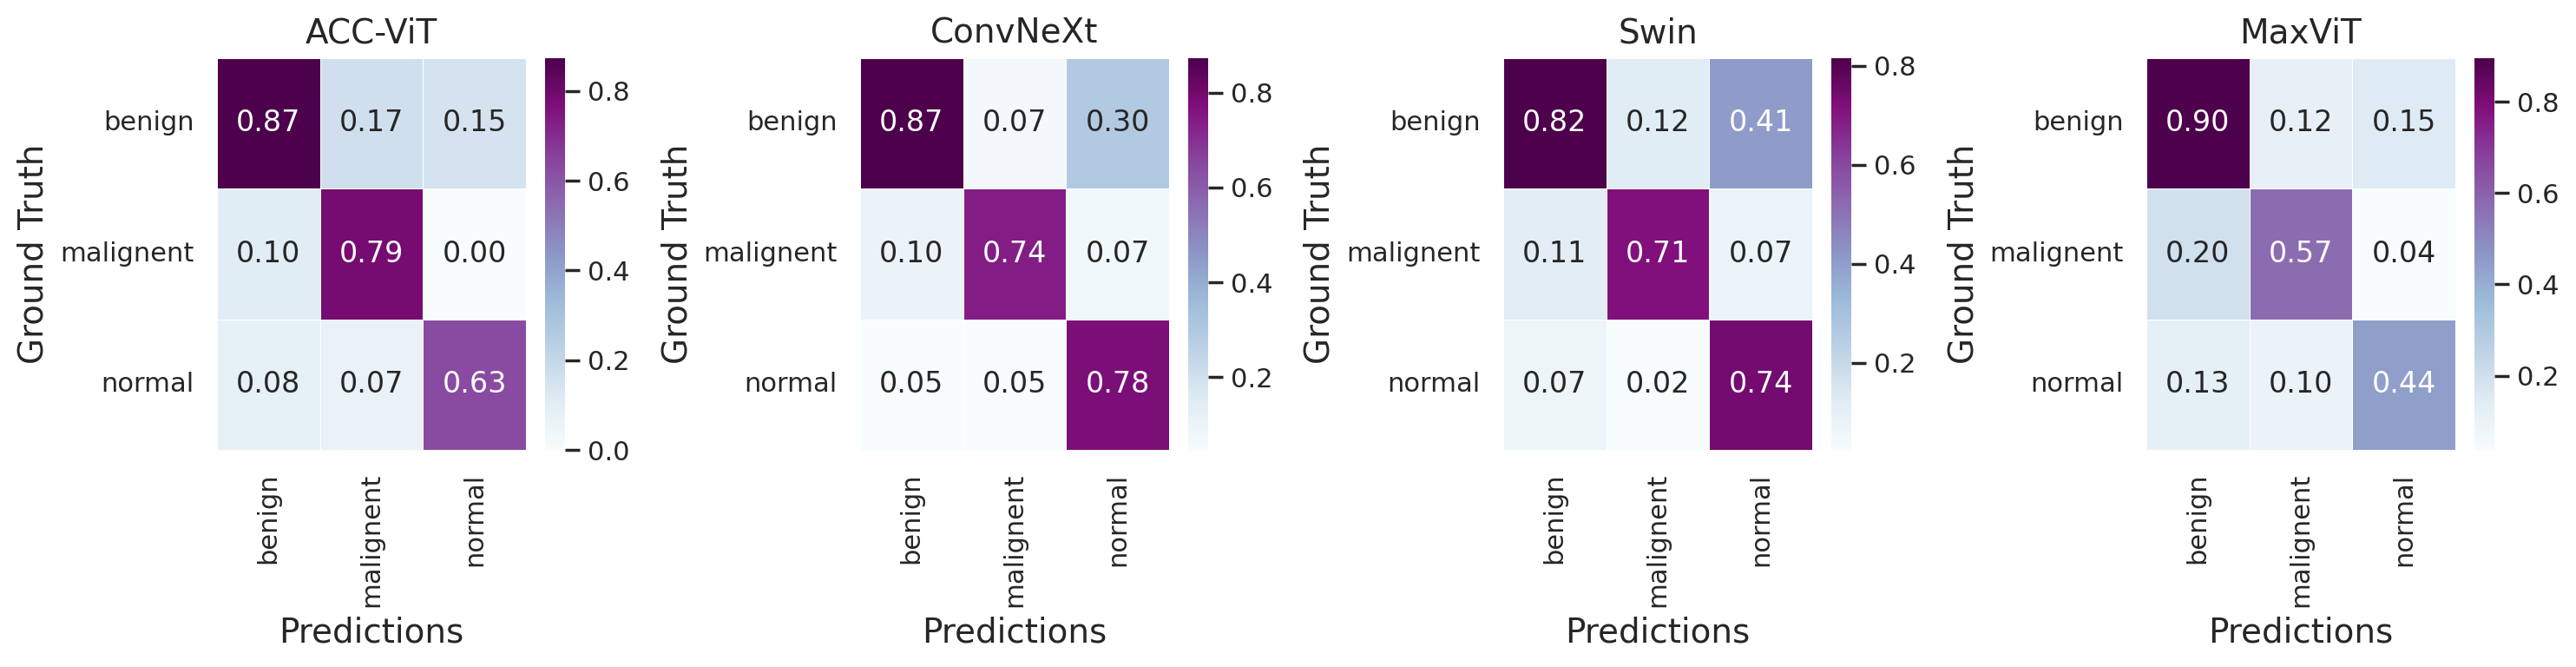}
         \caption{BUSI dataset}         
     \end{subfigure}
        \caption{Confusion Matrix of the different models on the three datasets.}
        \label{fig:three graphs}
\end{figure*}

\clearpage

\begin{table}[h]
\centering
\caption{Detailed results on the ELEVATER benchmark}
\label{tbl:szero}
\footnotesize
\begin{tabular}{c|cccc|cccc}
\hline
      & ACC-ViT  & MaxViT  & ConvNext  & SwinT   & ACC-ViT    & MaxViT  & ConvNext  & SwinT   \\ \hline
      & \multicolumn{4}{c|}{Caltech101}          & \multicolumn{4}{c}{HatefulMemes}         \\ \hline
exp 1 & 2.321   & 1.704   & 0.966     & 0.820   & 51.539    & 47.770  & 51.164    & 49.114  \\
exp 2 & 2.028   & 1.719   & 0.972     & 0.869   & 53.729    & 50.279  & 50.998    & 52.128  \\
exp 3 & 1.792   & 1.768   & 1.299     & 1.090   & 53.232    & 53.865  & 54.555    & 51.534  \\
mean  & 2.047   & 1.730   & 1.079     & 0.926   & 52.833    & 50.638  & 52.239    & 50.925  \\ \hline
      & \multicolumn{4}{c|}{CIFAR10}             & \multicolumn{4}{c}{KITTI}        \\\hline
exp 1 & 13.380  & 13.020  & 12.570    & 11.650  & 36.287    & 36.850  & 33.333    & 34.599  \\
exp 2 & 11.920  & 11.490  & 11.200    & 11.360  & 25.738    & 26.864  & 22.785    & 27.004  \\
exp 3 & 12.040  & 11.060  & 10.470    & 10.200  & 34.599    & 36.850  & 35.443    & 32.068  \\
mean  & 12.447  & 11.857  & 11.413    & 11.070  & 32.208    & 33.521  & 30.52     & 31.224  \\\hline
      & \multicolumn{4}{c|}{CIFAR100}            & \multicolumn{4}{c}{MNIST}                 \\\hline
exp 1 & 1.670   & 1.270   & 1.250     & 1.260   & 12.840    & 11.810  & 10.660    & 10.280  \\
exp 2 & 1.460   & 1.090   & 1.100     & 1.040   & 10.080    & 9.79    & 9.9       & 9.32    \\
exp 3 & 1.240   & 1.120   & 1.190     & 1.030   & 11.560    & 11.330  & 9.650     & 10.440  \\
mean  & 1.457   & 1.160   & 1.180     & 1.110   & 11.493    & 10.977  & 10.07     & 10.013  \\\hline
      & \multicolumn{4}{c|}{Country211}             & \multicolumn{4}{c}{OxfordFlowers}             \\\hline
exp 1 & 0.521   & 0.474   & 0.412     & 0.479   & 0.875     & 0.804   & 0.603     & 0.677   \\
exp 2 & 0.564   & 0.474   & 0.412     & 0.502   & 0.877     & 1.011   & 1.428     & 0.853   \\
exp 3 & 0.540   & 0.431   & 0.403     & 0.474   & 1.169     & 0.913   & 1.255     & 0.632   \\
mean  & 0.542   & 0.46    & 0.409     & 0.485   & 0.974     & 0.909   & 1.095     & 0.721   \\\hline
      & \multicolumn{4}{c|}{DescriTextures}                 & \multicolumn{4}{c}{OxfordPets}      \\\hline
exp 1 & 3.564   & 2.128   & 2.021     & 2.447   & 2.428     & 3.822   & 3.078     & 2.581   \\
exp 2 & 2.713   & 2.553   & 1.915     & 2.340   & 2.570     & 3.909   & 2.352     & 2.978   \\
exp 3 & 1.968   & 2.340   & 2.128     & 2.5     & 3.112     & 3.868   & 3.914     & 2.298   \\
mean  & 2.748   & 2.340   & 2.021     & 2.429   & 2.703     & 3.866   & 3.115     & 2.619   \\ \hline
      & \multicolumn{4}{c|}{EuroSAT}        & \multicolumn{4}{c}{PatchCamelyon}         \\\hline
exp 1 & 15.020  & 12.520  & 14.980    & 11.520  & 53.110    & 49.261  & 49.863    & 50.766  \\
exp 2 & 11.260  & 11.340  & 11.020    & 12.720  & 50.455    & 51.105  & 50.897    & 53.296  \\
exp 3 & 12.900  & 13.220  & 12.740    & 13.800  & 50.577    & 47.644  & 49.640    & 49.203  \\
mean  & 13.060  & 12.360  & 12.913    & 12.680  & 51.381    & 49.337  & 49.640    & 51.088  \\\hline
      & \multicolumn{4}{c|}{FER2013}             & \multicolumn{4}{c}{Rendered SST2}         \\\hline
exp 1 & 17.526  & 16.551  & 17.080    & 13.291  & 49.918    & 49.918  & 50.082    & 50.137  \\
exp 2 & 17.164  & 17.693  & 14.015    & 16.244  & 50.082    & 50.082  & 50.082    & 49.918  \\
exp 3 & 14.322  & 13.848  & 13.514    & 13.987  & 50.082    & 50.632  & 49.918    & 50.192  \\
mean  & 16.337  & 16.031  & 14.87     & 14.507  & 50.027    & 50.211  & 50.027    & 50.082  \\ \hline
      & \multicolumn{4}{c|}{FGVC Aircraft} & \multicolumn{4}{c}{RESISC45}         \\ \hline
exp 1 & 1.030   & 1.121   & 0.970     & 0.965   & 2.742     & 3.040   & 1.853     & 1.615   \\
exp 2 & 1.120   & 1.302   & 1.029     & 1.255   & 2.155     & 2.357   & 1.679     & 1.877   \\
exp 3 & 1.667   & 1.210   & 1.273     & 1.087   & 2.758     & 2.964   & 1.921     & 1.889   \\
mean  & 1.272   & 1.211   & 1.091     & 1.102   & 2.552     & 2.787   & 1.818     & 1.794   \\ \hline
      & \multicolumn{4}{c|}{Food 101}            & \multicolumn{4}{c}{Stanford Cars}           \\ \hline
exp 1 & 0.820   & 1.398   & 0.764     & 1.022   & 0.609     & 0.336   & 0.597     & 0.348   \\
exp 2 & 1.469   & 2.079   & 0.950     & 1.224   & 0.609     & 0.497   & 0.560     & 0.410   \\
exp 3 & 1.465   & 0.994   & 0.859     & 1.552   & 0.597     & 0.597   & 0.659     & 0.560   \\
mean  & 1.251   & 1.49    & 0.858     & 1.266   & 0.605     & 0.477   & 0.605     & 0.439   \\ \hline
      & \multicolumn{4}{c|}{GTSRB}               & \multicolumn{4}{c}{VOC2007} \\\hline
exp 1 & 2.090   & 2.937   & 3.325     & 3.135   & 18.129    & 16.195  & 17.851    & 17.208  \\
exp 2 & 1.655   & 1.401   & 1.283     & 2.082   & 17.238    & 16.639  & 16.050    & 17.618  \\
exp 3 & 2.391   & 1.314   & 1.805     & 2.621   & 19.410    & 17.173  & 16.351    & 16.663  \\
mean  & 2.045   & 1.884   & 2.138     & 2.613   & 18.259    & 16.669  & 16.751    & 17.163 \\\hline
\end{tabular}
\end{table}

\clearpage
